# Supplementary material for: AGS-Mesh: Adaptive Gaussian Splatting and Meshing with Geometric Priors for Indoor Room Reconstruction Using Smartphones
Source: arXiv:2411.19271 source file (2024-12-16)
Supplement: Supplementary file 1 [file supp_mesh_figs.tex]

\newcommand*\rot{\rotatebox{90}}
\newcommand{\fourwidth}{0.236\textwidth}

\begin{figure*}[t!]
    \centering
    \setlength{\tabcolsep}{0.1em}
    \renewcommand{\arraystretch}{0.8}
    \hfill{}\hspace*{-0.5em}
    \footnotesize
    \begin{tabular}{ccccc}
            \rot{\qquad\qquad\quad Reference}&
            \includegraphics[width=\fourwidth]{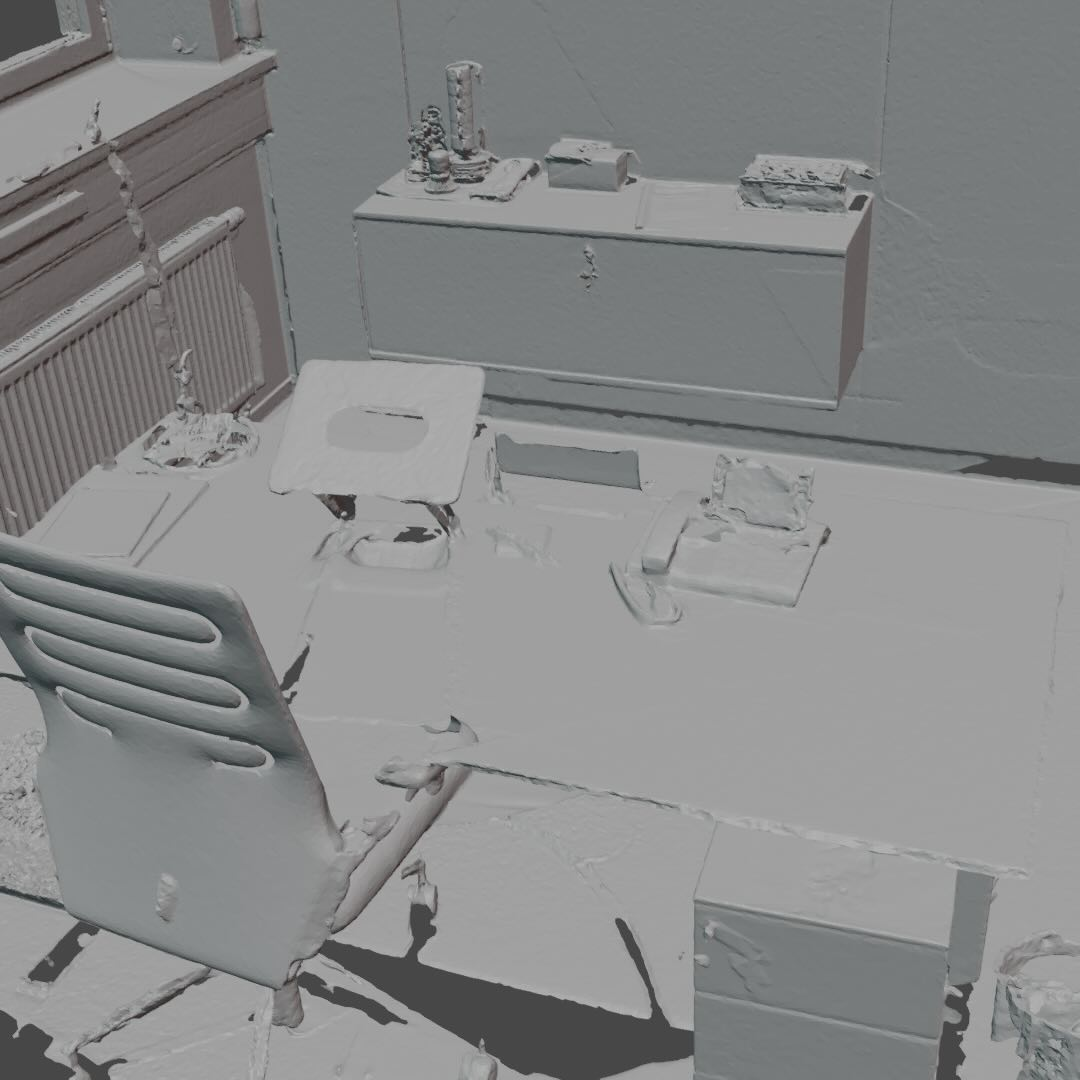}&
            \includegraphics[width=\fourwidth]{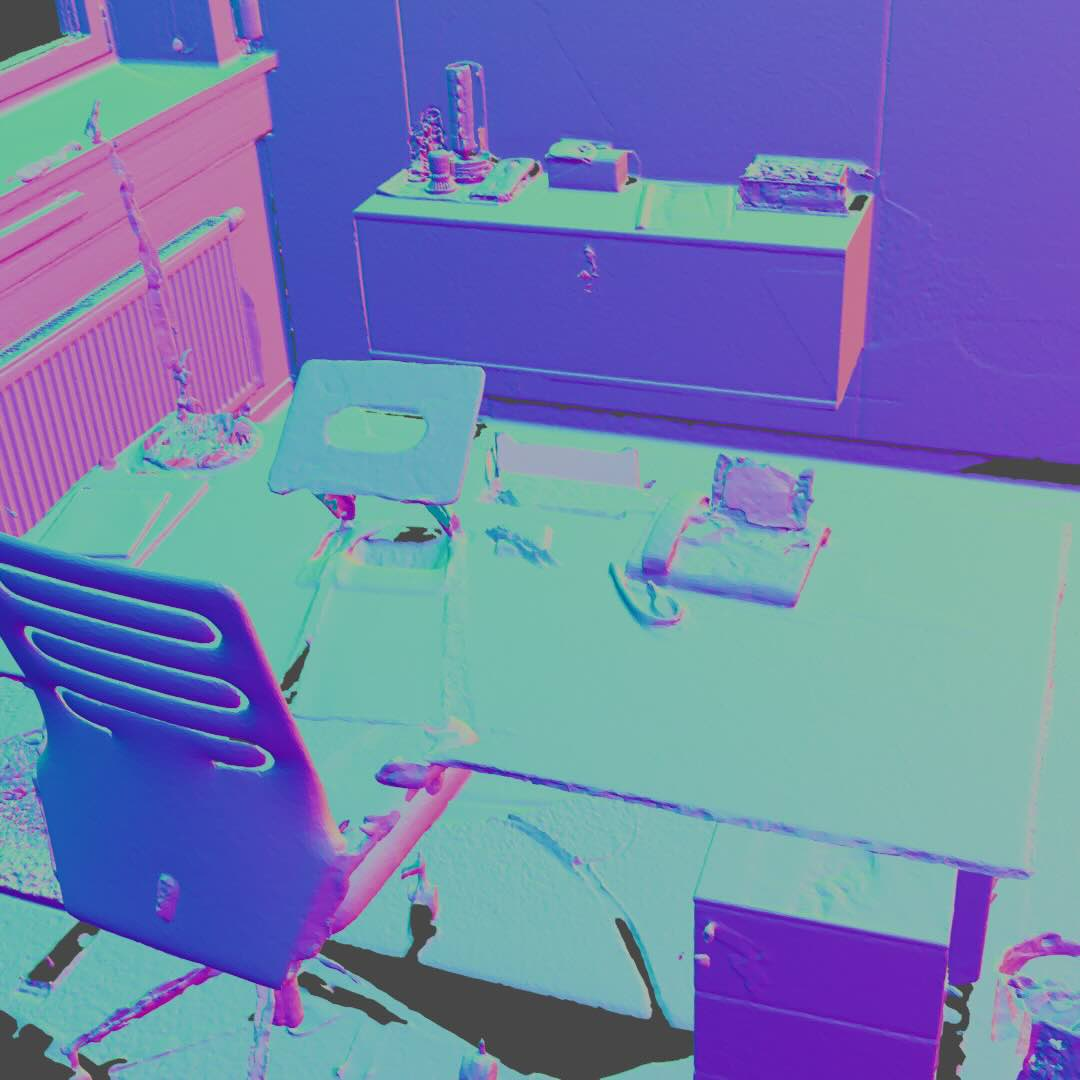}&
            \includegraphics[width=\fourwidth]{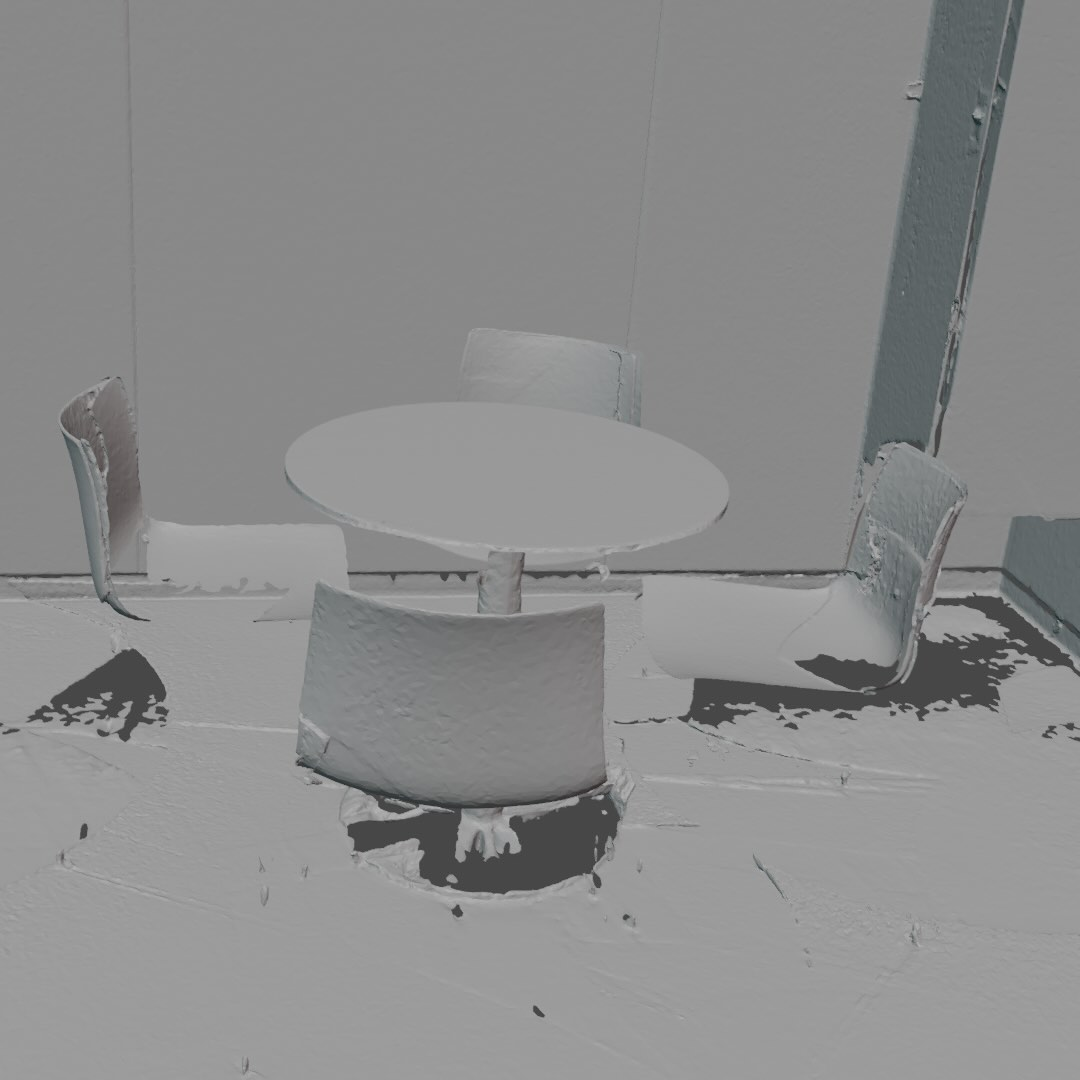}&
            \includegraphics[width=\fourwidth]{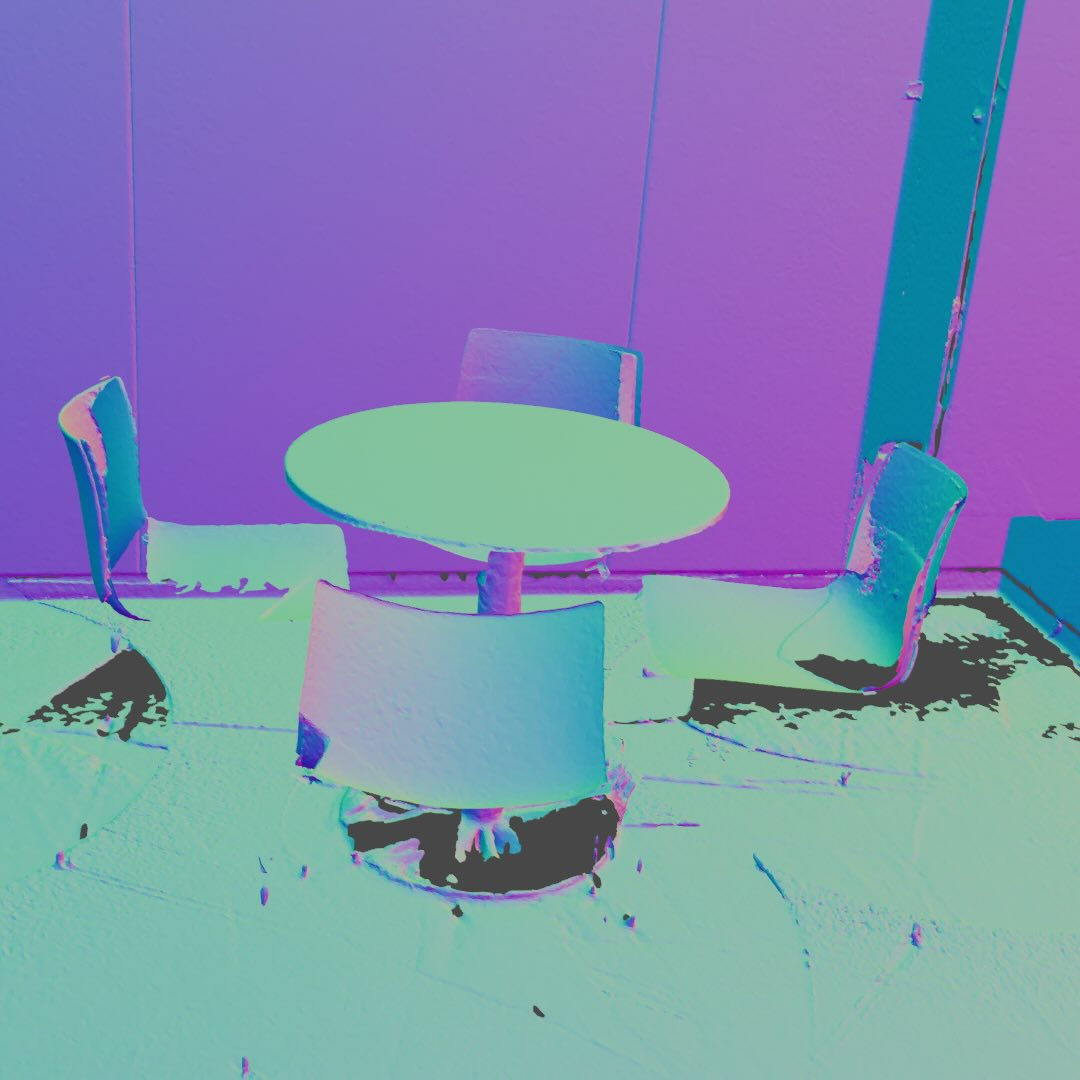}
            \\
            \rot{\qquad\qquad Splatfacto~\cite{nerfstudio}}&
            \includegraphics[width=\fourwidth]{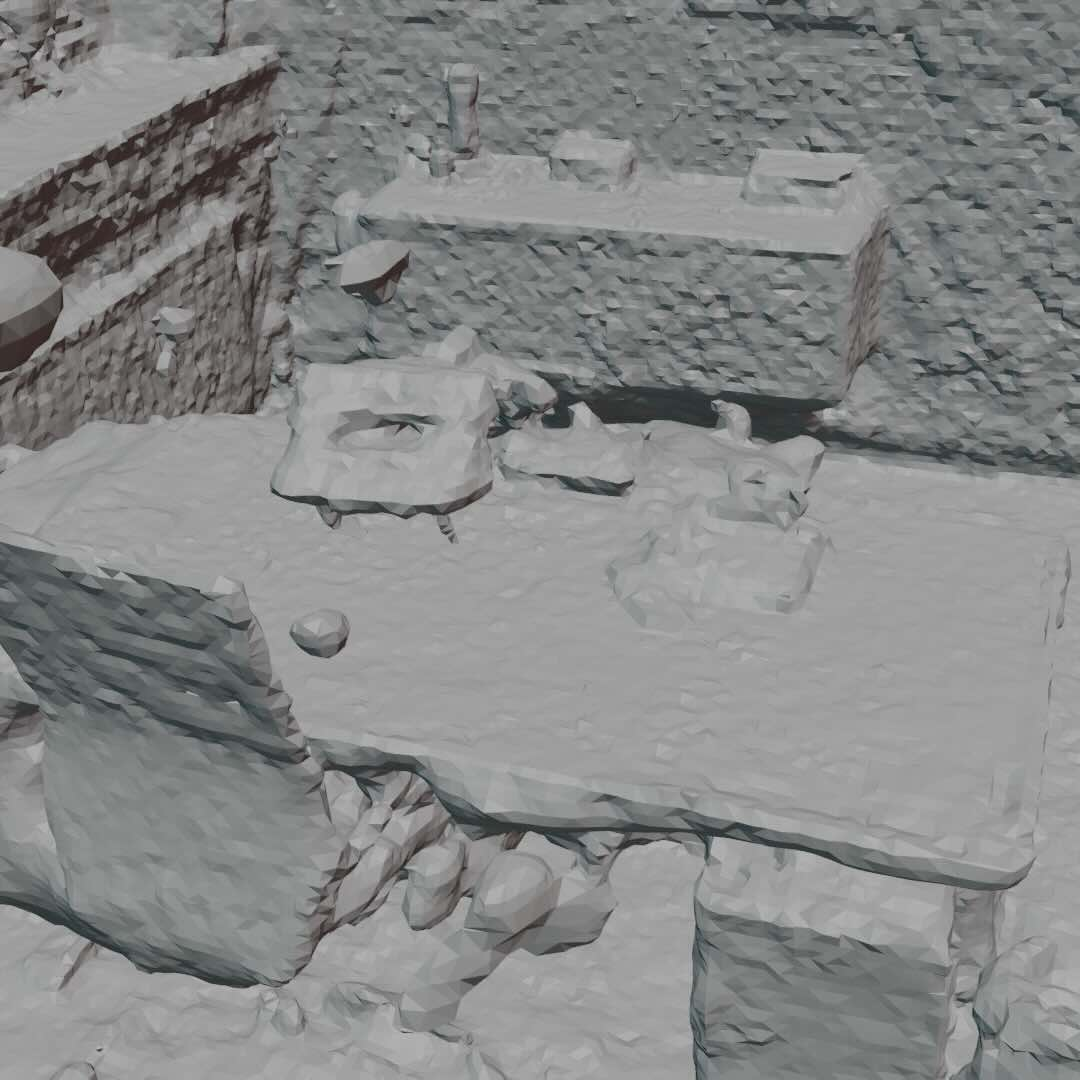}&
            \includegraphics[width=\fourwidth]{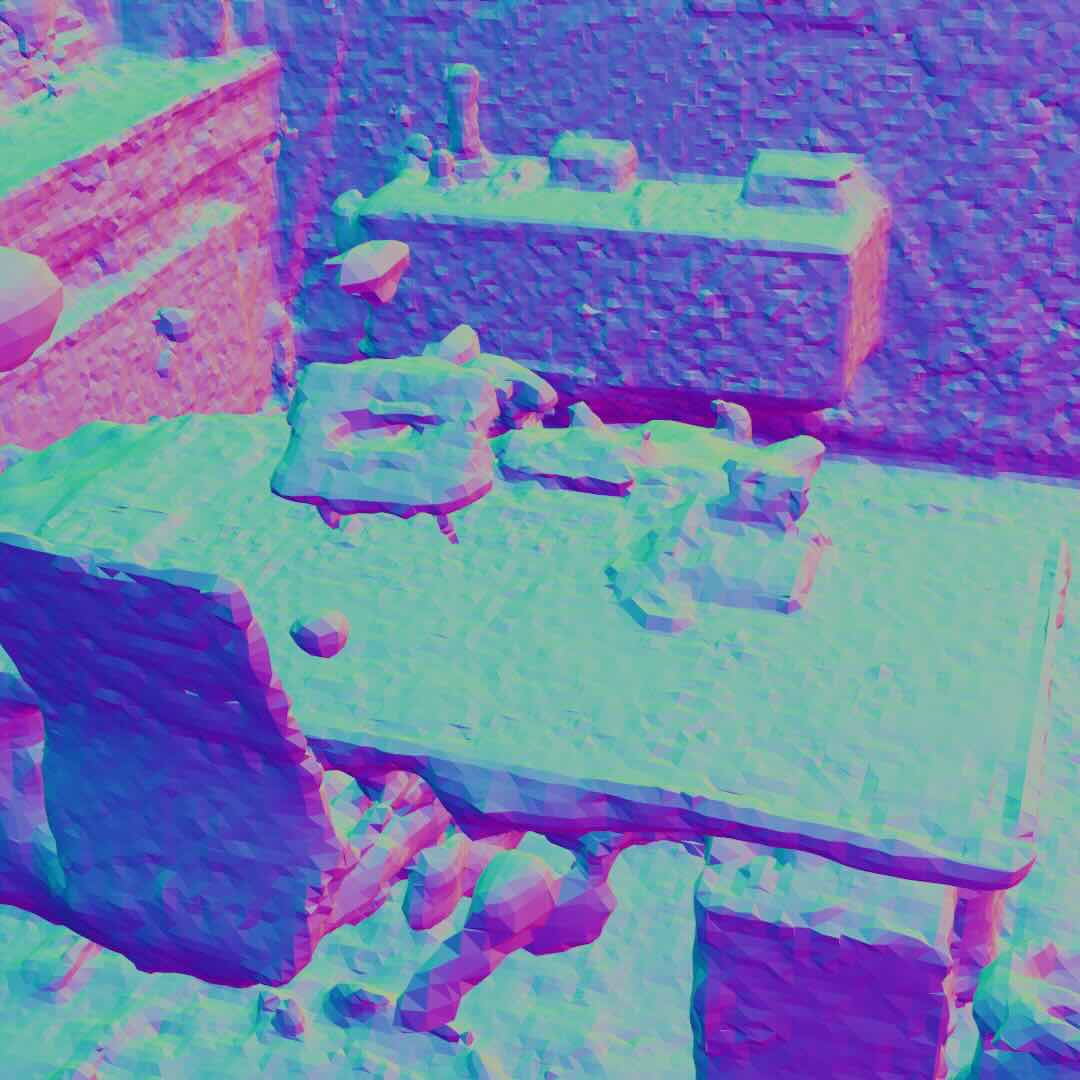}&
            \includegraphics[width=\fourwidth]{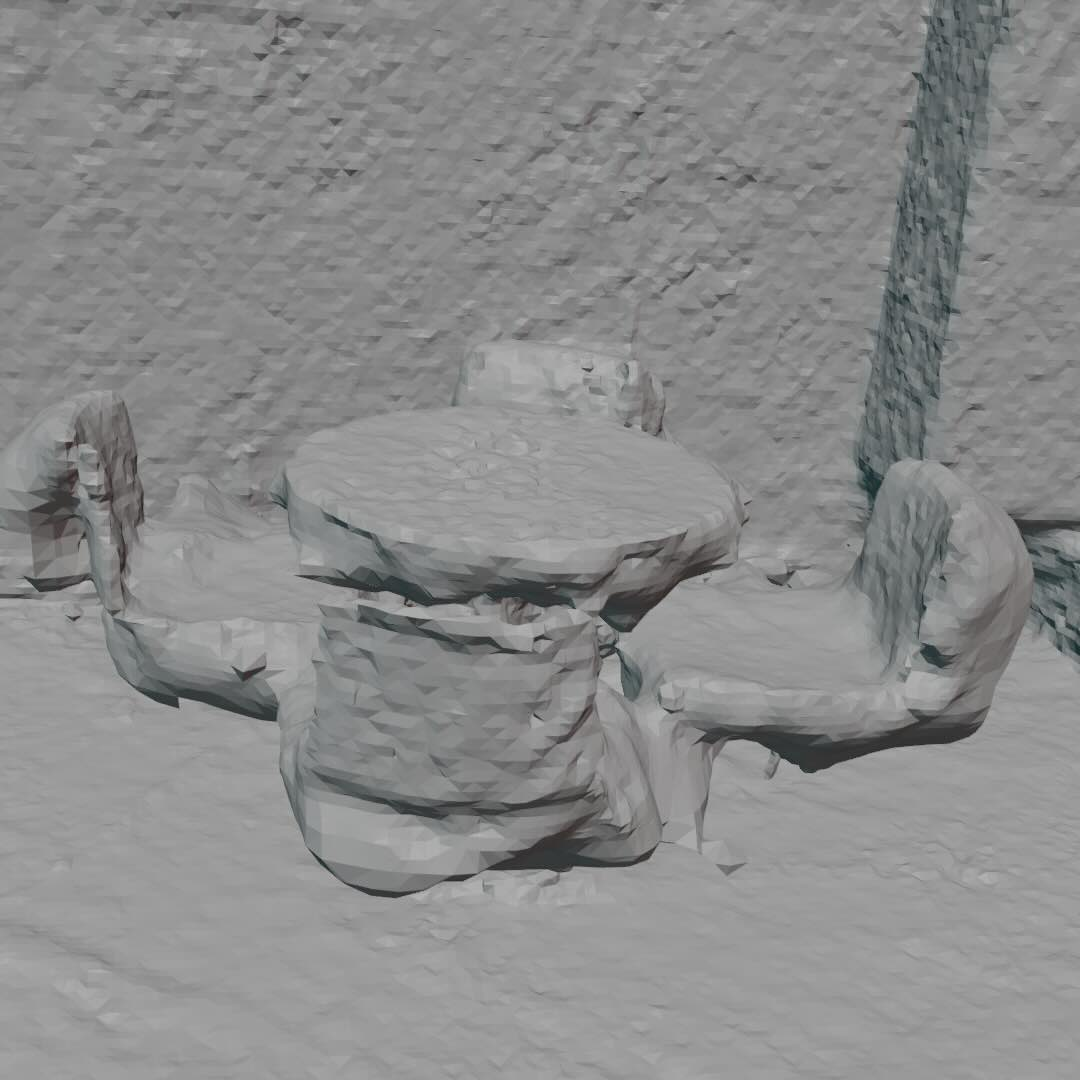}& \includegraphics[width=\fourwidth]{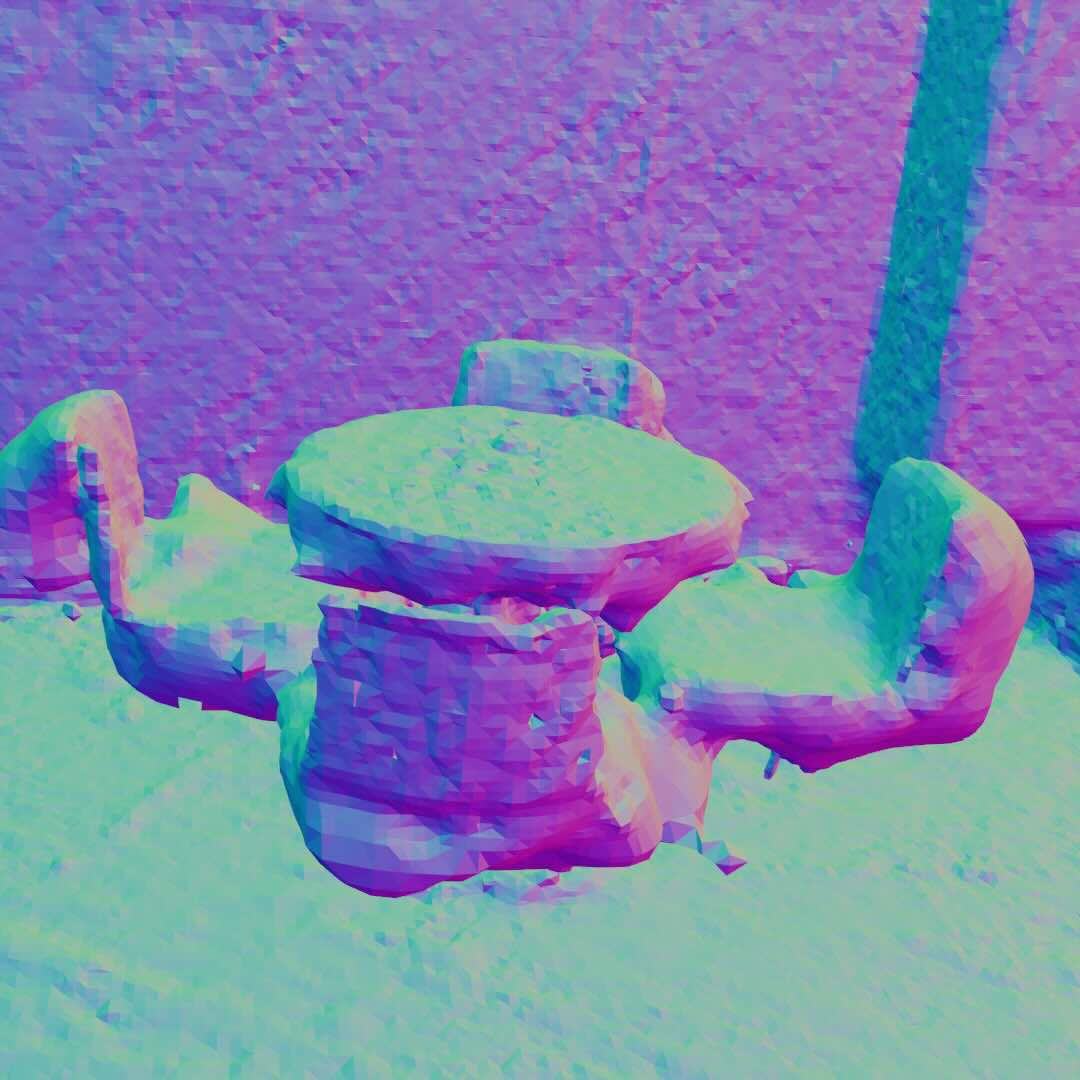}
            \\
            \rot{\qquad DN-Splatter~\cite{turkulainen2024dn} + Ours}&
            \includegraphics[width=\fourwidth]{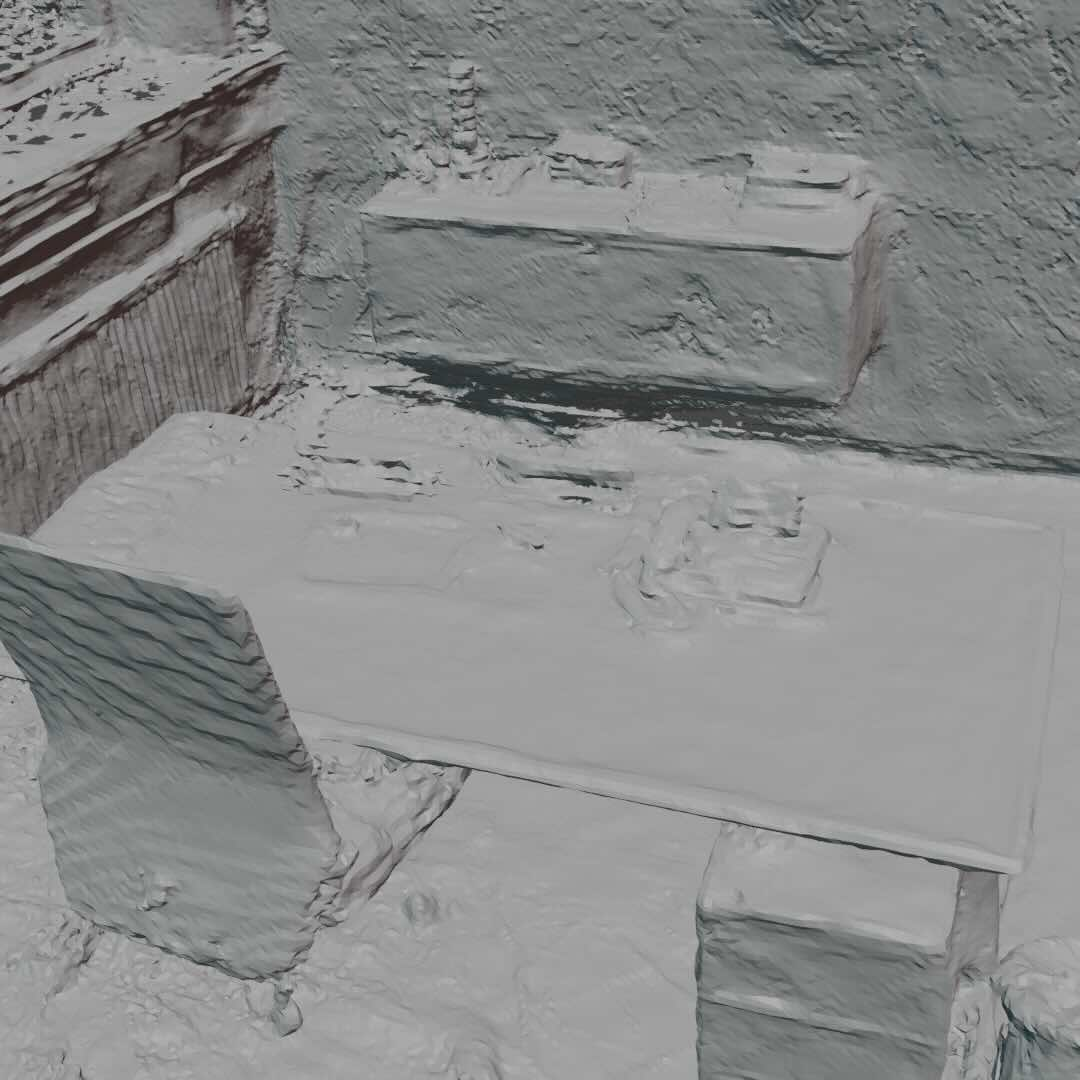}&
            \includegraphics[width=\fourwidth]{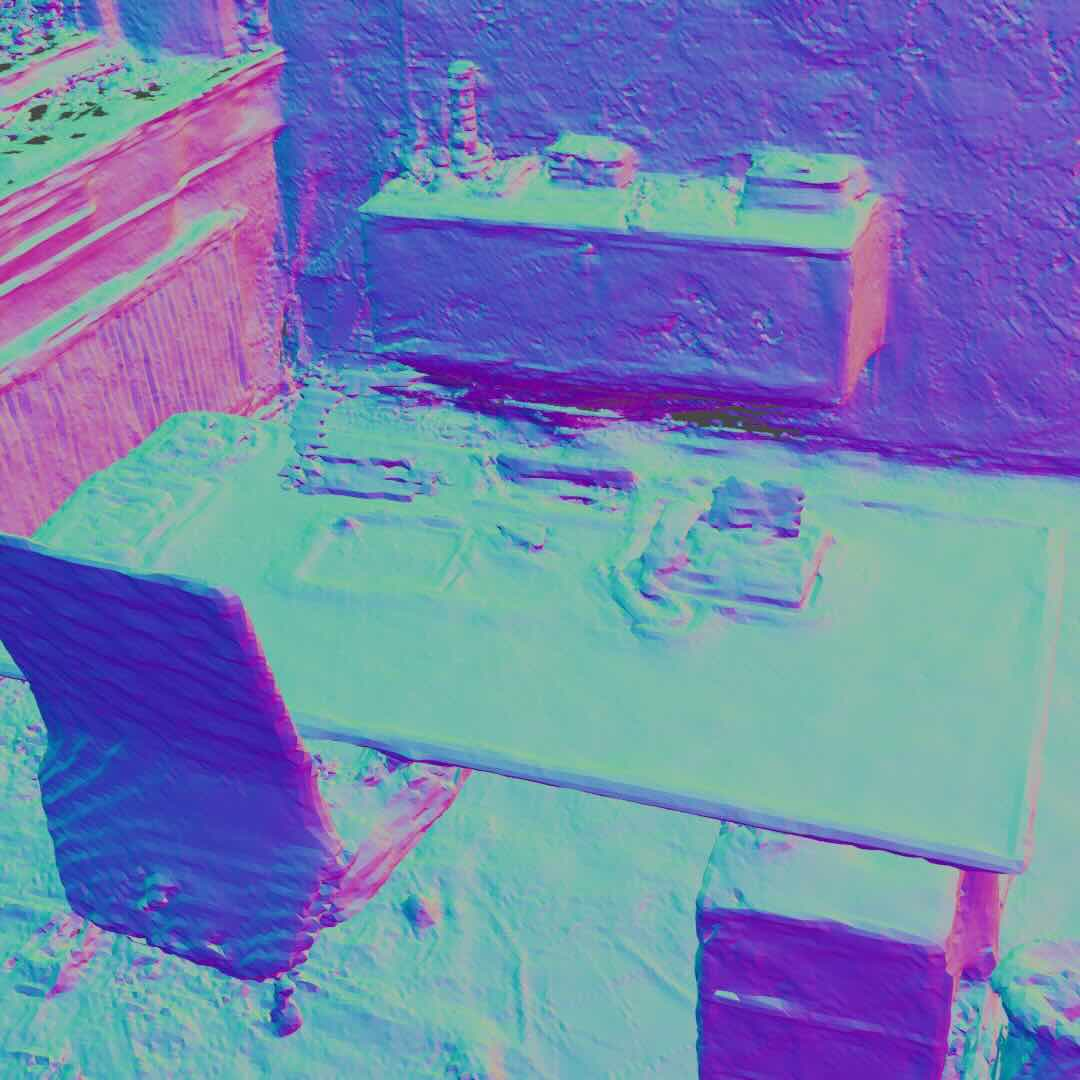}&
            \includegraphics[width=\fourwidth]{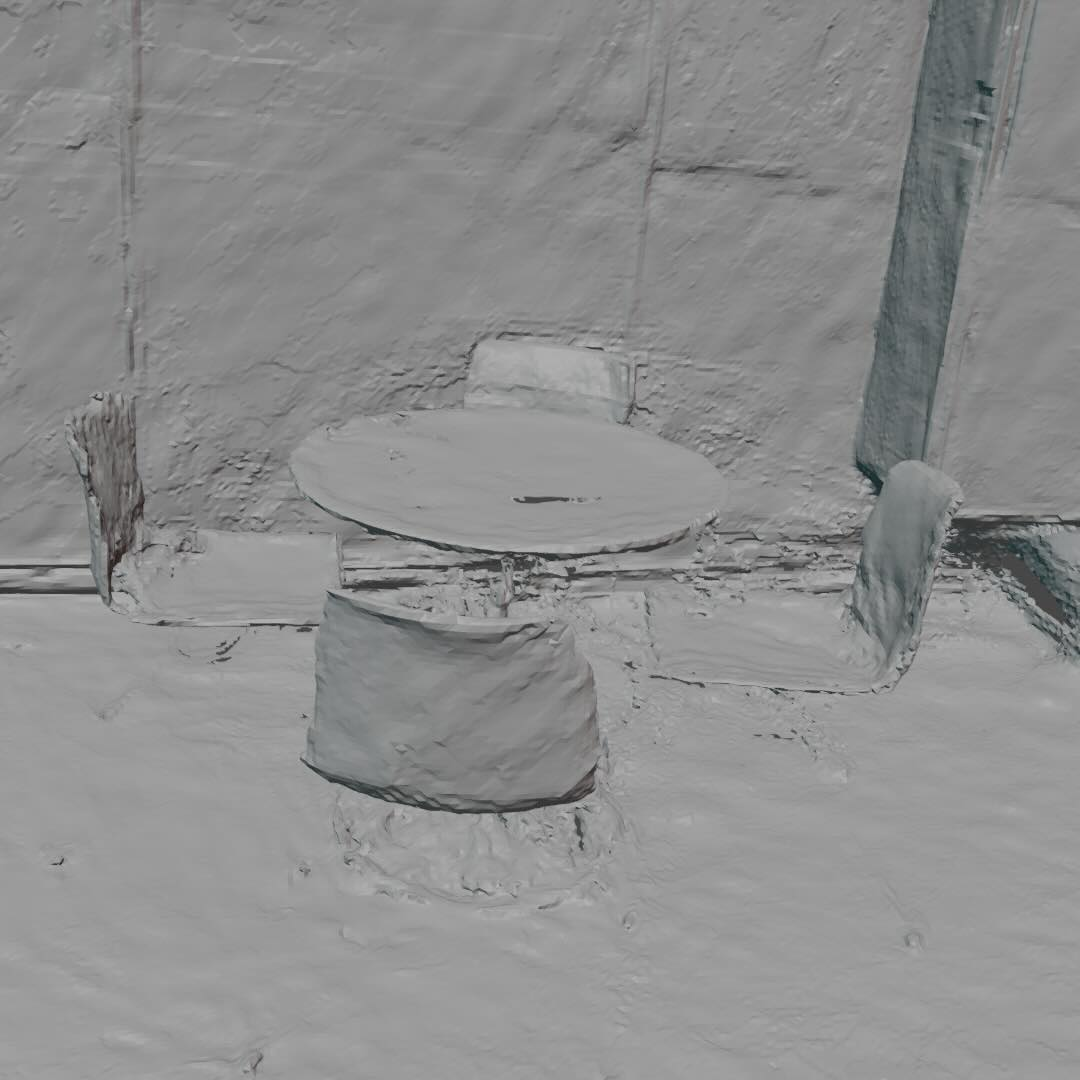}& \includegraphics[width=\fourwidth]{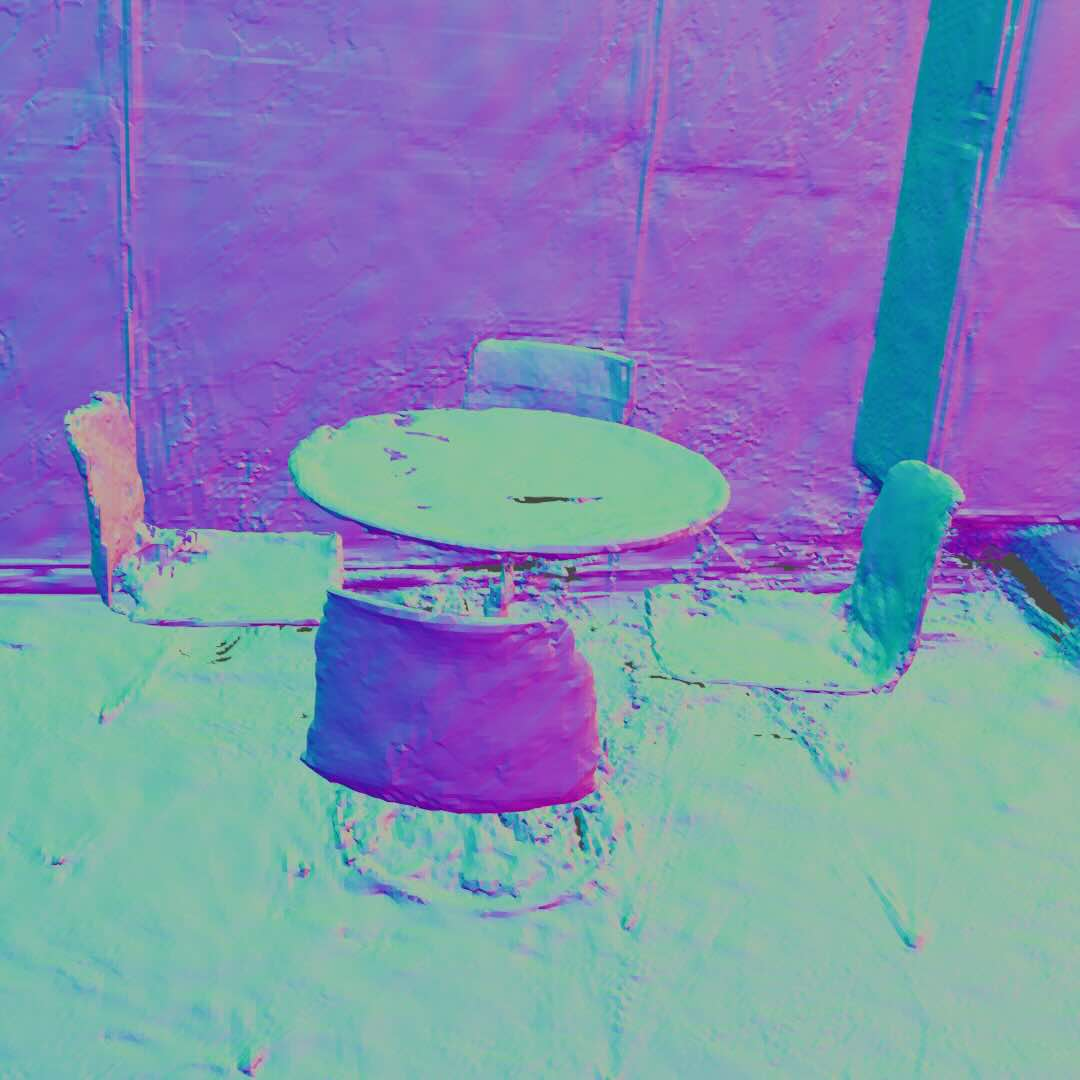}
            \\
            \rot{\qquad\qquad 2DGS~\cite{Huang2DGS2024}}&
            \includegraphics[width=\fourwidth]{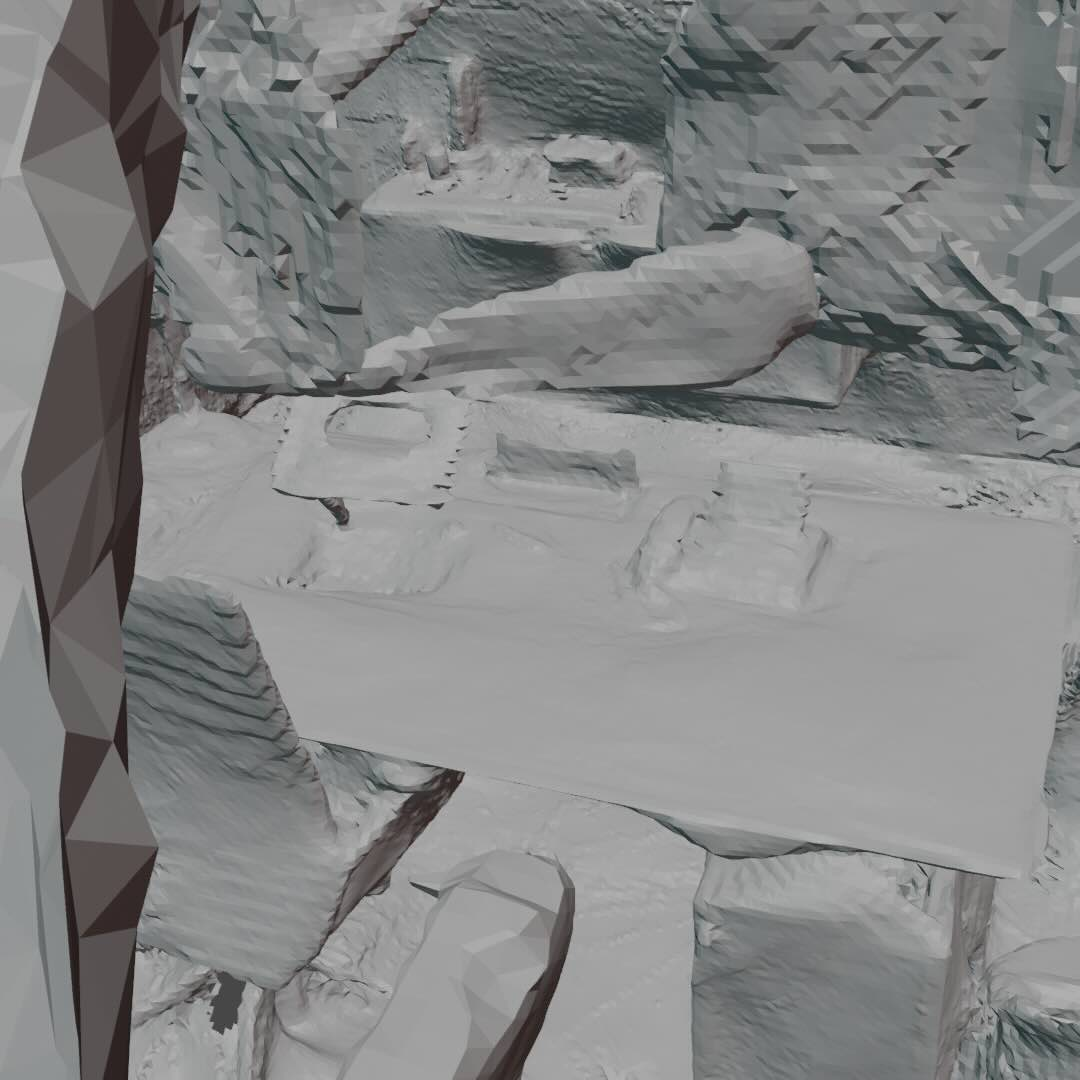}&
            \includegraphics[width=\fourwidth]{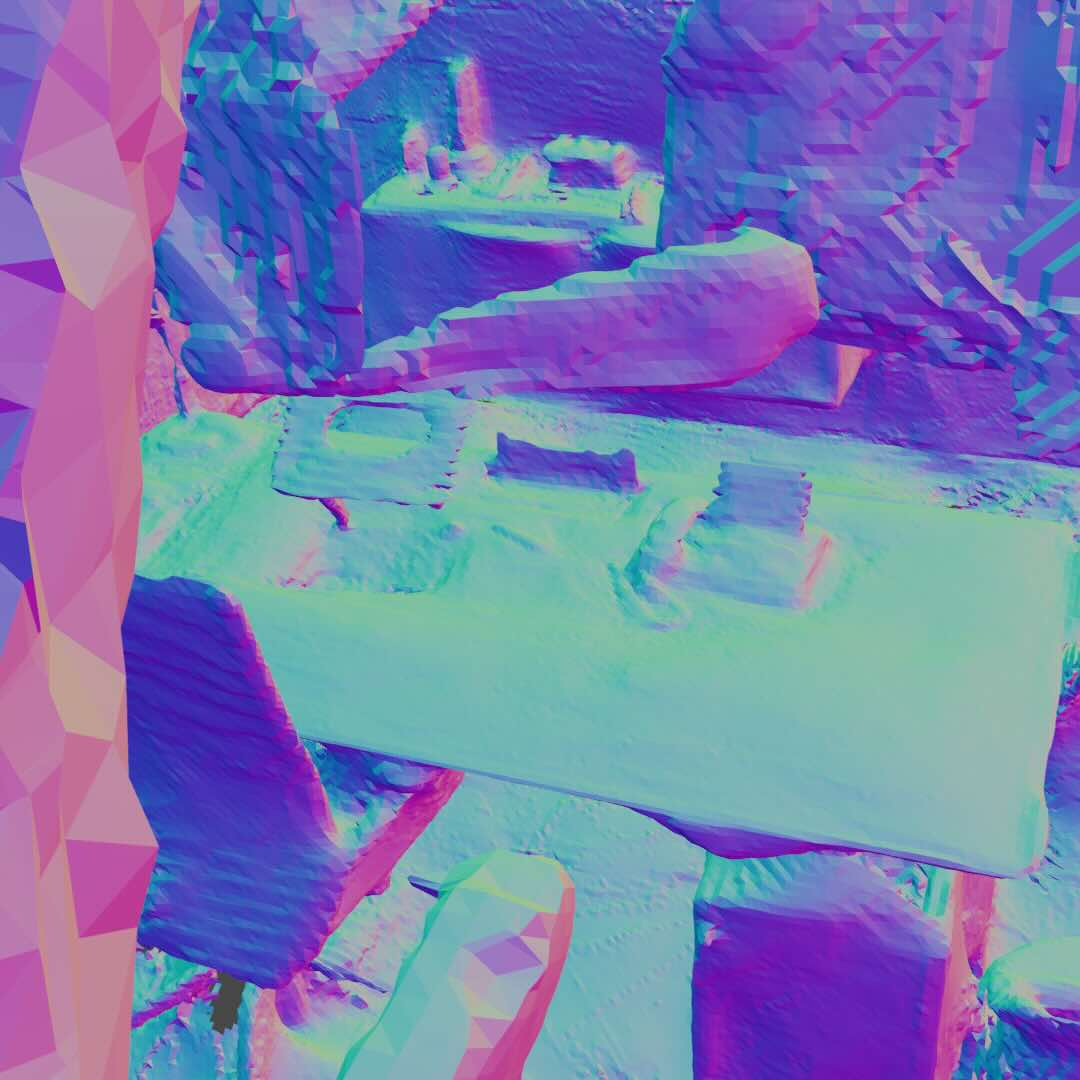}&
            \includegraphics[width=\fourwidth]{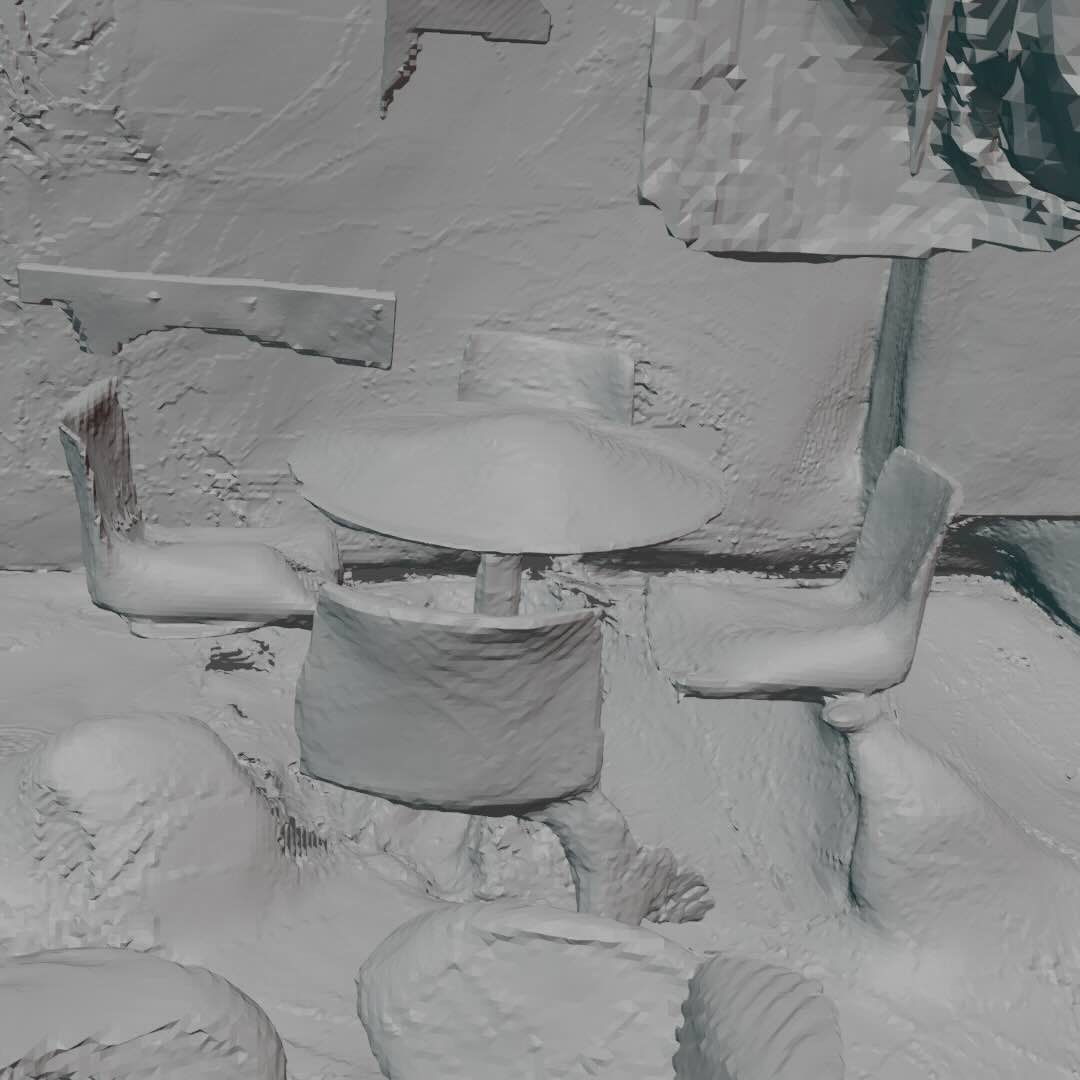}& \includegraphics[width=\fourwidth]{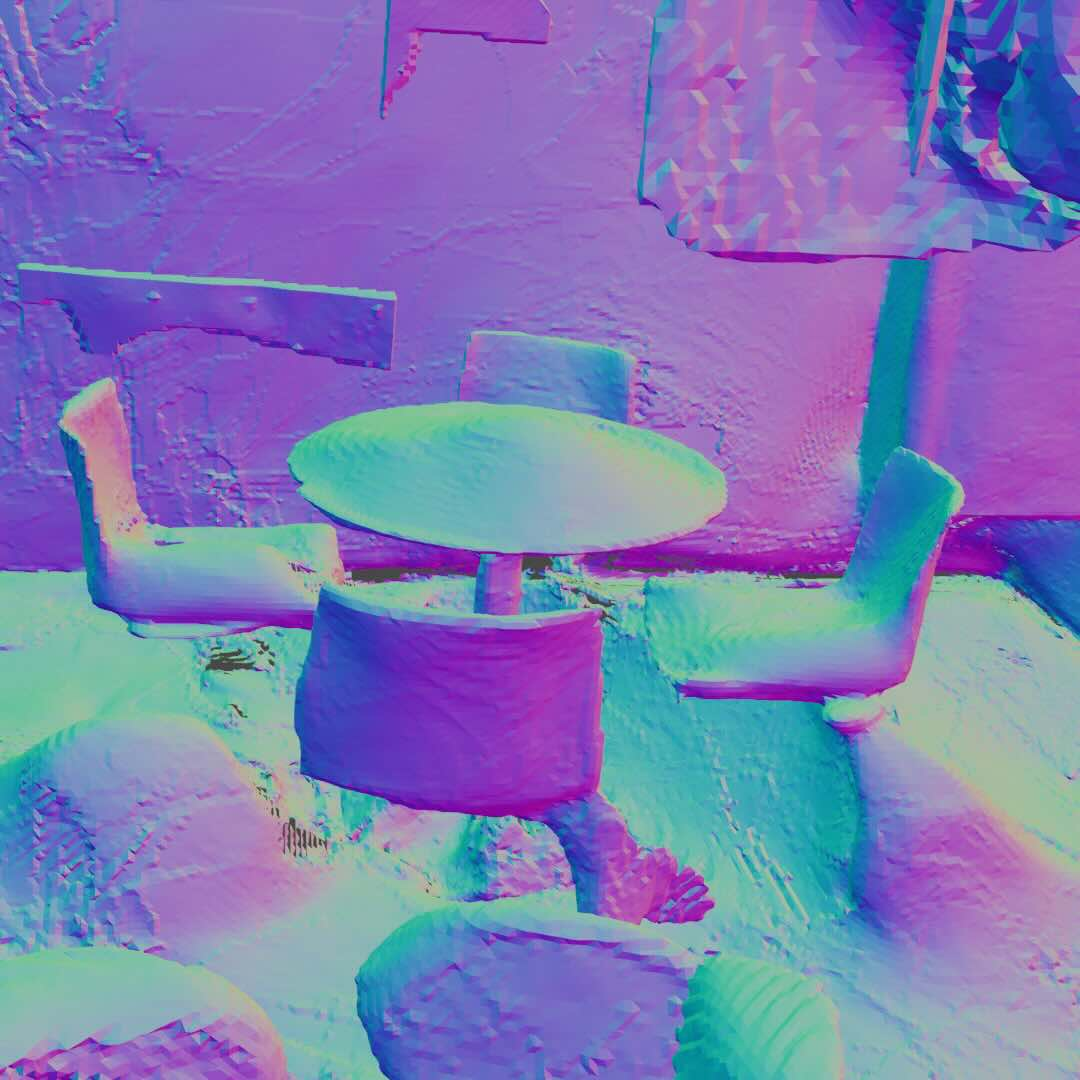}
            \\
            \rot{\qquad\qquad 2DGS~\cite{Huang2DGS2024} + Ours}&
            \includegraphics[width=\fourwidth]{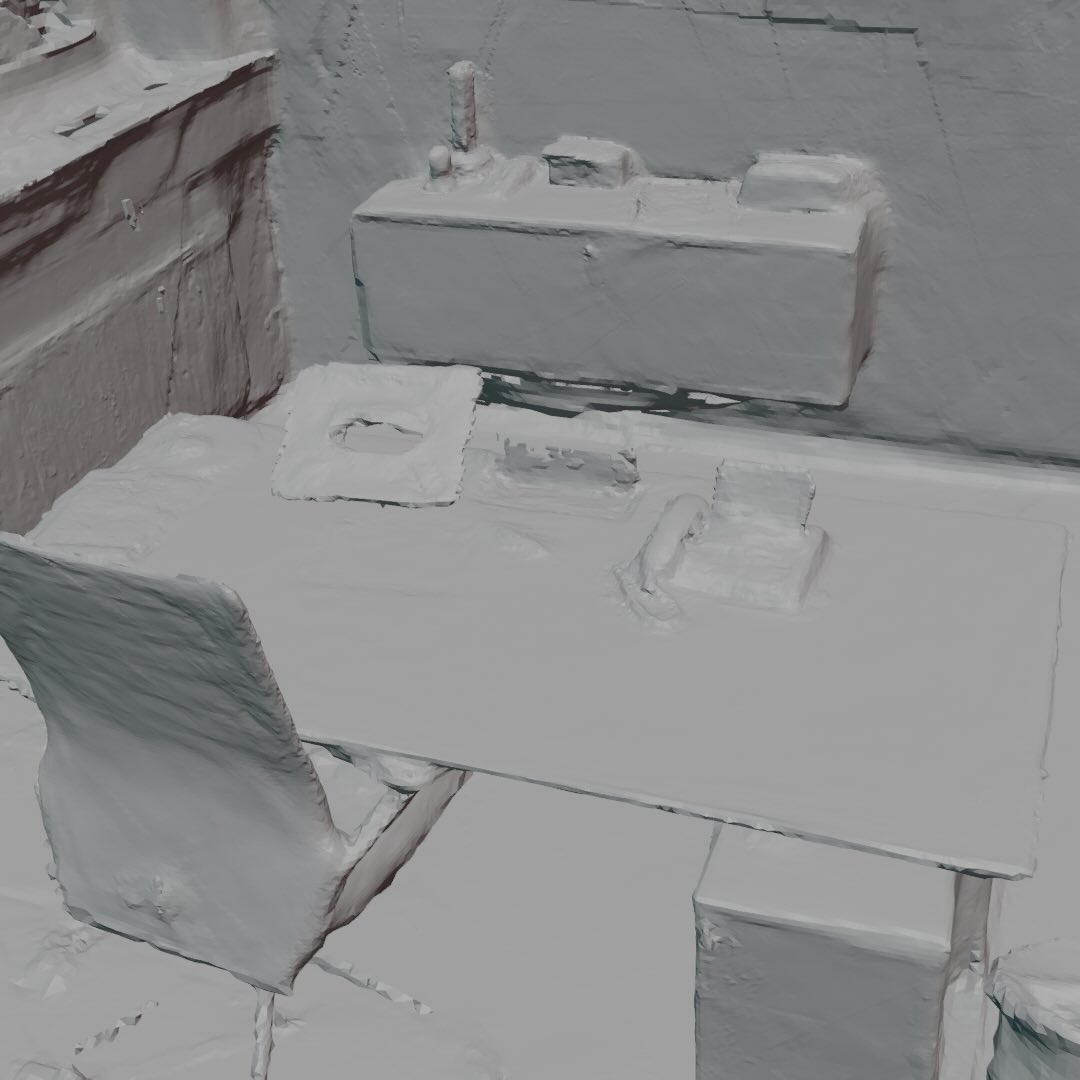}&
            \includegraphics[width=\fourwidth]{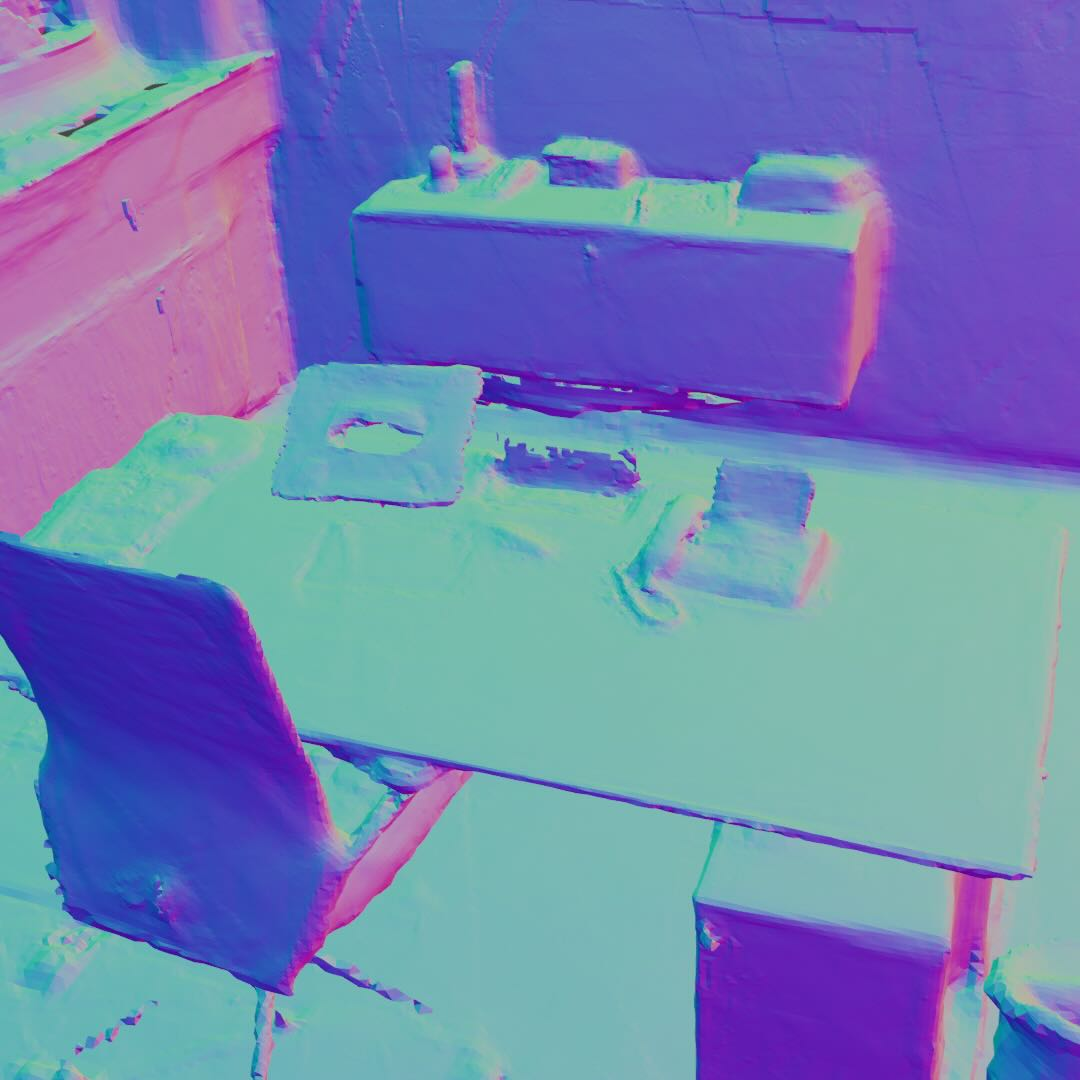}&
            \includegraphics[width=\fourwidth]{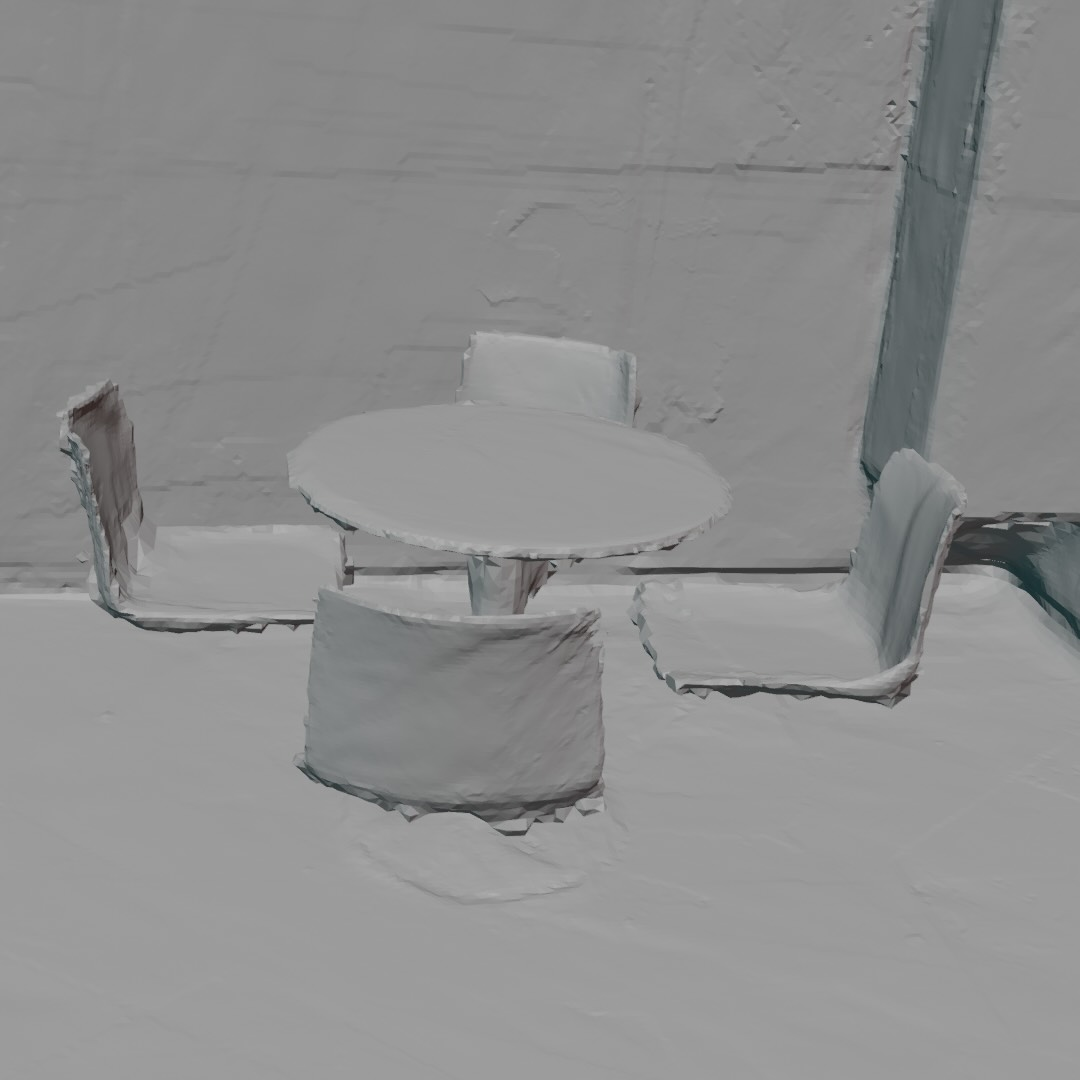}& \includegraphics[width=\fourwidth]{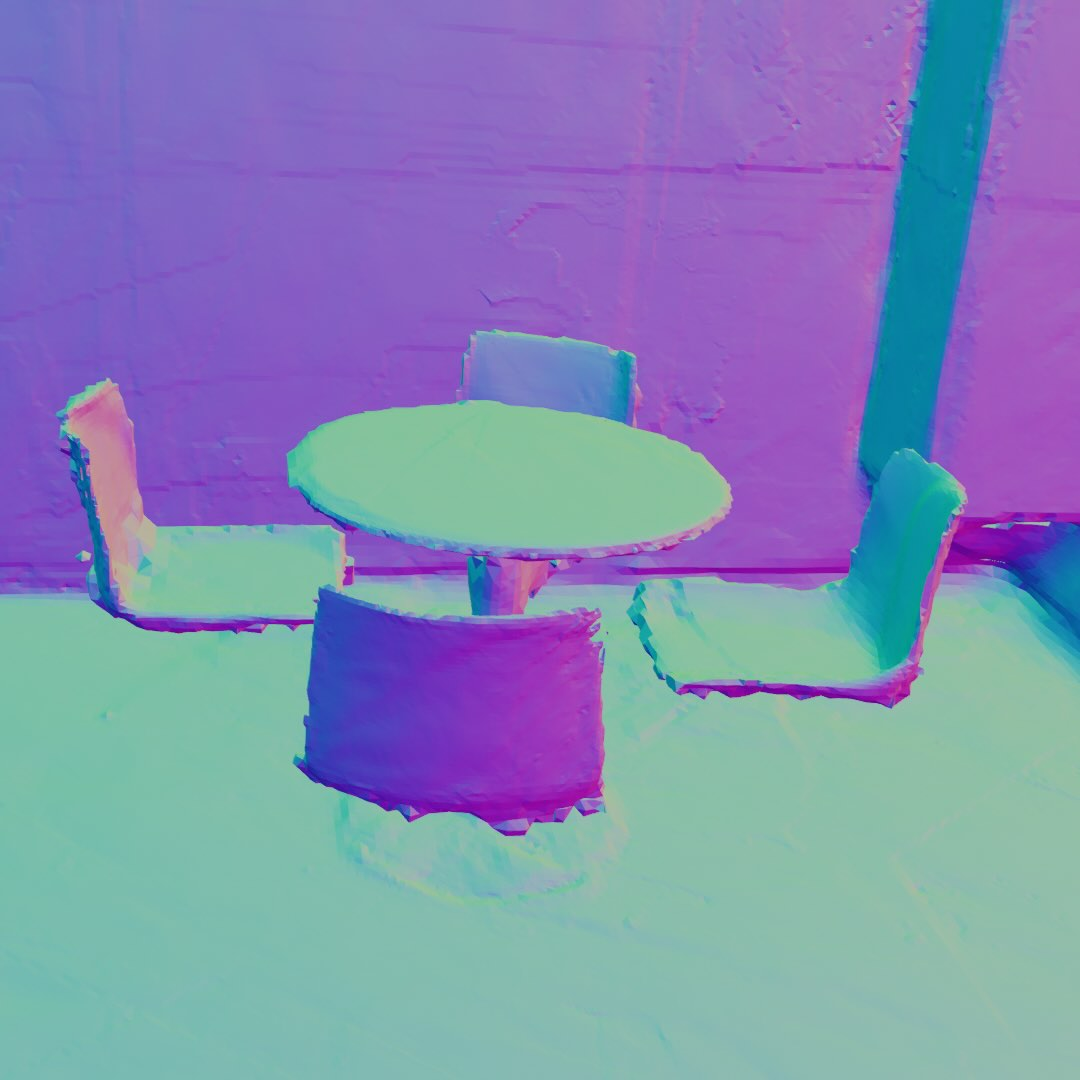}
    \end{tabular}
  \caption{Qualitative mesh comparison for the "8b5caf3398" scene from ScanNet++ dataset.}
  \label{fig:scannetpp-cmp}
\end{figure*}
